# Supplementary material for: Grow and Merge: A Unified Framework for Continuous Categories Discovery
Source: arXiv:2210.04174 source file (2022-10-09)
Supplement: Supplementary file 1 [file A_metrics.tex]

\setcounter{table}{0}   %从0开始编号，显示出来表会A1开始编号
\setcounter{figure}{0}
\setcounter{equation}{0}
%定义编号格式，在数字序号前加字符“A"

% \renewcommand{\theequation}{A.\arabic{equation}}

\section{Evaluation Metrics}
\label{apendix:metrics}
% cluster acc
% forgetting
% discovery
At each time-step $t$, we evaluate the classification performance on the test dataset $\mathcal{D}^t_{test} = \{  (\bm{x}_i^s, y_i^s) | s \leq t     \}$, containing test samples from all the known or previously discovered categories.
For the newly appeared unknown categories, we evaluate the novel category discovery performance.
% The categories $\mathcal{C}^t = \{  1, \cdots, K^t \}$ in which $\mathcal{D}^t_{train}$ is drawn from contain both the already-learned categories $\{  1, \cdots, K^{t-1} \}$ and the novel categories $\{ K^{t-1}+1, \cdots, K^t \}$.

At the end of the continuous learning stage, we design the \textbf{maximum forgetting metric} $\mathcal{M}_f$ and the \textbf{final discovery metric} $\mathcal{M}_d$ for evaluation.
$\mathcal{M}_f$ measures the capability to maintain the performance on the known categories, which is the lower the better.
$\mathcal{M}_d$ measures the ability to discover novel categories, which is the higher the better.
To evaluate the performance of the clustering assignments, we follow the standard practise~\cite{han2021autonovel, drncd} to adopt clustering accuracy.
First, an optimal permutation $h^*$ that matches the cluster assignments $y_i^*$ with the ground truth label $y_i$ is obtained by solving the following optimization problem using Hungarian algorithm~\cite{kuhn1955hungarian}: 
\begin{align}
    h_t^* = \mathop{\arg\min}\limits_{h} \frac{1}{M^t} \sum_{i=1}^{M^t} \mathbb{I}(y_i=h(y_i^*)),
\end{align}
where $M^t$ denotes the size of $\mathcal{D}_{test}^t$. 
The clustering accuracy on the known categories $\text{ACC}_{\text{known}}^t$ and novel categories $\text{ACC}_{\text{novel}}^t$ at time $t$ can be obtained as follows: 
\begin{align}
    \text{ACC}_{\text{known}}^t &= \frac{1}{M_{\text{known}}^t} \sum_{i=1}^{M_{\text{known}}^t}\mathbb{I} (  y_{i,\text{known}} = h_t^*(y_i^*) ),\\ 
    \text{ACC}_{\text{novel}}^t &= \frac{1}{M_{\text{novel}}^t} \sum_{i=1}^{M_{\text{novel}}^t}\mathbb{I} (  y_{i,\text{novel}} = h_t^*(y_i^*) ),
\end{align}
where $M_{\text{known}}^t$ and $M_{\text{novel}}^t$ denote the number of known category samples and novel category samples from $\mathcal{D}_{test}^t$, respectively.
The $y_{i,\text{known}}$ and $y_{i,\text{novel}}$ denote the label of the known samples and category samples, respectively.
Then, the maximum forgetting $\mathcal{M}_f$ and final discovery $\mathcal{M}_d$ can be obtained by 
\begin{align}
    \mathcal{M}_f &= \max_t \{ \text{ACC}_{\text{known}}^0 - \text{ACC}_{\text{known}}^t \},\\
    \mathcal{M}_d &= \text{ACC}_{\text{novel}}^T.
\end{align}
The importance of $\mathcal{M}_f$ and $\mathcal{M}_d$ are different.
First, $\mathcal{M}_f$ should be sufficiently low, otherwise a model forgetting the previous learned tasks is not practically useful in the real world applications.
Second, the model should improve $\mathcal{M}_d$ as much as possible on the condition of low $\mathcal{M}_f$.
