# Supplementary material for: Grow and Merge: A Unified Framework for Continuous Categories Discovery
Source: arXiv:2210.04174 source file (2022-10-09)
Supplement: Supplementary file 2 [file C_scenario.tex]

\setcounter{table}{0}   %从0开始编号，显示出来表会A1开始编号
\setcounter{figure}{0}
\setcounter{equation}{0}
%定义编号格式，在数字序号前加字符“A"

\section{Scenarios Details}
\label{appendix:scen}
We formulate four different scenarios for experiments as follows:

\textit{Class Incremental Scenario (CI)}: the data are only drawn from the novel categories, \ie, $\mathcal{C}^t \cap ( \mathcal{C}^{t-1} \cup \cdots \cup \mathcal{C}^0  )=\emptyset, \forall t\in\{ 1, \cdots, T  \}$.
CI is a standard scenario that only requires the models to learn from the novel samples and keep the performance of the known categories.

\textit{Data Incremental Scenario (DI)}: the data are only drawn from the known categories, \ie, $\mathcal{C}^0= \mathcal{C}^t, \forall t\in \{1, \cdots, T\}$. 
DI is a simple scenario, which evaluates the models' capability to improve the feature representation with the continuous unlabeled data. 

\textit{Mixed Incremental Scenario (MI)}: the data are drawn from both novel categories and the known categories, \ie, $\mathcal{C}^0\subset \mathcal{C}^1 \subset \cdots \subset \mathcal{C}^T$.
MI is more complicated than CI, where models are further required to identify whether the data comes from novel categories or not.

\textit{Semi-supervised Mixed Incremental Scenario (SMI)}: the data are drawn from both novel categories and the known categories, \ie, $\mathcal{C}^0\subset \mathcal{C}^1 \subset \cdots \subset \mathcal{C}^T$, and a portion of the data are labeled.
SMI is closer to the real-world application, where both labeled and unlabeled samples are provided in the incremental stages. 

For CI, 70\%/10\%/10\%/10\% classes of the CIFAR-100,  CUB-200 and ImageNet-100 datasets are used in the initial stage and the following 3 time-steps of the continuous category discovery stage, respectively.
For DI, 25\% of the data are used for the initial stage, and 75\% are used for the continuous category discovery stage, with 25\% data at each time-step.
For MI, 87\% data from 0-70 classes in CIFAR-100 are used for initial stage. 
7\% of data from 0-70 classes, 70\% data from 70-80 classes are used for $t=1$ during the continuous category discovery stage.
2\% data from 0-70 classes, 20\% data from 70-80 classes and 90\% data from 80-90 classes are used for $t=2$.
3\% data form 0-70 classes, 10\% data from 70-80 classes, 10\% data from 80-90 classes and all of the data from 90-100 classes are used during $t=3$.
For SMI, 20\% of the data from MI are labeled during $t=1,2,3$.
