# Supplementary material for: Grow and Merge: A Unified Framework for Continuous Categories Discovery
Source: arXiv:2210.04174 source file (2022-10-09)
Supplement: Supplementary file 4 [file B_construction.tex]

\setcounter{table}{0}   %从0开始编号，显示出来表会A1开始编号
\setcounter{figure}{0}
\setcounter{equation}{0}
%定义编号格式，在数字序号前加字符“A"

\section{Exemplar Set Construction}
After the initial pre-training stage, the exemplar set is initialized, following iCaRL~\cite{icarl}.
Denote $P_k=\{  \bm{p}_{k,i} \}_i$ as the exemplar set of the $k$-th class.
Then $\bm{p}_{k,i}$ is selected by solving the following optimization problem,
\begin{align}
    \bm{p}_{k,i} \longleftarrow \mathop{\arg\min}\limits_{{\bm{x}}_i^0} \left|\left| \frac{1}{N_k^0}\sum_{y_i^0=k}\phi_D^0 ( {\bm{x}}_i^0) - \frac1j [\phi_D^0 ( {\bm{x}}_i^0) + \sum_{s=1}^{k-1} \phi_D^t ( \bm{p}_{k,s} )    ] \right|\right|,
\end{align}
where $N_k^0$ denotes the number of samples belong to the $k$-th class.
