# Supplementary material for: Grow and Merge: A Unified Framework for Continuous Categories Discovery
Source: arXiv:2210.04174 source file (2022-10-09)
Supplement: Supplementary file 6 [file D_implemetation.tex]

\setcounter{table}{0}   %从0开始编号，显示出来表会A1开始编号
\setcounter{figure}{0}
\setcounter{equation}{0}
%定义编号格式，在数字序号前加字符“A"

\section{Implementation Details}
\label{appendix:impl}
For all experiments, we use ResNet-18~\cite{resnet18} network as the encoder, and fully connected layers as the classifier and the cluster head. 
SGD optimizer~\cite{sgd} with learning rate 0.1, momentum 0.9 and weight decay $1e-4$ is used. 
The learning rate decays for every 60 epochs.
The batch size is set to 128 for CIFAR-100 dataset, 64 for CUB-200 dataset and 32 for ImageNet-100.
All the experiments run on the platform with Intel Xeon CPU E5-2640 and Nvidia GeForce RTX 3080 GPUs.
